# Supplementary material for: BANG: Billion-Scale Approximate Nearest Neighbor Search using a Single GPU
Source: arXiv:2401.11324 source file (2025-04-12)
Supplement: Supplementary file 1 [file appendix.tex]

\section{Appendix: Prior Work}
\label{c:app1}

Original version of GPU$\_$ANN was implemented, prior to start of this thesis work, at the Microsoft Research. Besides the CPU code, it consists of following 6 kernels:

\begin{enumerate}
\item Prepare$\_$PQ$\_$Dist$\_$Table: Computes the distances of all centroids from the query vectors, and populates the PQ Dist Table.
\item Filter$\_$Neighbors: Filters out the neighbors, already received in the prior iterations. 
\item Calculate$\_$Neighbor$\_$Distance: For every query, computes the distance between the neighbors and the query through lookups to
the PQ Dist Table and the compressed vectors of the neighbors.
\item Sort$\_$Neighbor$\_$Array: For every query, sort the neighbors in increasing order of their distances to the query.
\item Merge$\_$LSet: Merge the current Best L Set (candidate set) with the sorted neighbors to update the candidate
set.
\item Re-ranking: Computes the exact L2 distances of the candidate nodes with the query nodes for re-ranking.
\end{enumerate}

The CPU code, in addtion to acting as the driver, performs one other task: compiling the parent's neighbor IDs and communicate them to GPU. We denote this CPU task in italics in the code's outline.\\
The outline of the code is shown below-

\begin{algorithm2e}
\DontPrintSemicolon % Some LaTeX compilers require you to use \dontprintsemicolon instead 
Prepare$\_$PQ$\_$Dist$\_$Table()\;
\Repeat{Stopping$\_$Criteria() }{
  \textit{Compile$\_$Neighbor$\_$IDs()}\;
  Filter$\_$Neighbors()\;  
  Calculate$\_$Neighbor$\_$Distance()\; 
  Sort$\_$Neighbor$\_$Array()\; 
  Merge$\_$LSet()\; 
}
Re-rank()\;

\caption{{\sc Outline} }
\label{algo:outline2}
\end{algorithm2e}
 
\subsection{Kernel Details}
\subsubsection{Prepare$\_$PQ$\_$Dist$\_$Table}
The distance computation is parallelized across queries, and within a query, it is parallelized across centroids.
The total number of threads are divided into equal-sized groups called thread-block. A thread-block is assigned
to a query. The work/computations specific to a query are performed by the block of threads assigned to it.
Now within a query, the threads of a thread-block compute the distance of the chunks to the 256 centroids in
parallel.\\

\subsubsection{Filter$\_$Neighbors}
The neighbor filtering is parallelized across queries, and within a query it is parallelized across neighbors. The work specific to a query is performed by the thread block assigned to it. A single neighbor ID is given to each thread which in turn indexes into the bloom filter to decide if the neighbor should be filtered out or not. If neighbor is not filtered out, it is added to new neighbors array using atomic operation on GPU memory.

\subsubsection{Calculate$\_$Neighbor$\_$Distance}
The distance computation is parallelized across queries, and within a query it is parallelized across neighbors.
Here again, a thread-block is assigned to a query. Within a query, a group of threads compute the distance of
one neighbor to the query, in a cooperative manner.
The kernel is bounded by the I/O due to the lookup based distance computation. The primary bottleneck in
this kernel is the lookup of the distances of the centroids of the compressed vectors in the PQ Dist Table, which are
arbitrary and lack locality. Thus, the accesses to the PQ Dist Table and the compressed vectors are uncoalesced.
The irregularity in accesses cannot be removed completely. It may be reduced by changing the index graph
layout.

\subsubsection{Sort$\_$Neighbor$\_$Array}
The sorting is parallelized across queries.
Within a query, the sorting of the neighbors based on their distances to the query is parallelized using \verb|parallel merge sort|.
One thread-block sorts the neighbors of a query.
The implementation is at par with the best-in-class comparison based parallel sorting algorithms for floatingpoint values. It also makes use of the GPU memory hierarchy to reduce the memory latency.

\subsection{Merge$\_$LSet}
The merging is parallelized across queries.
For a query, the merging of the candidate set and the neighbors is parallelized using a parallel merge algorithm
for merging sorted arrays using binary search.
One thread-block merges the neighbors of a query to its candidate set.
The implementation exploits the memory hierarchy to reduce memory latency

\subsubsection{Re-rank}
The L2 distance computation is parallelized.
One thread-block computes the L2 distances of the candidate nodes with the query using the full-precision
coordinates
